# Supplementary material for: Frustration-induced emergent Hilbert space fragmentation
Source: arXiv:2011.01936 source file (2021-06-16)

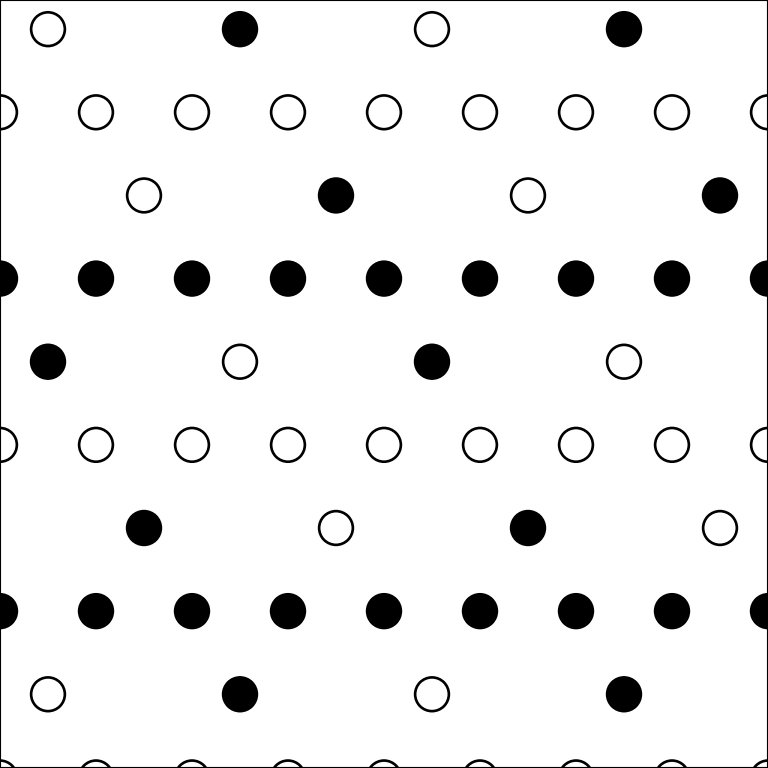

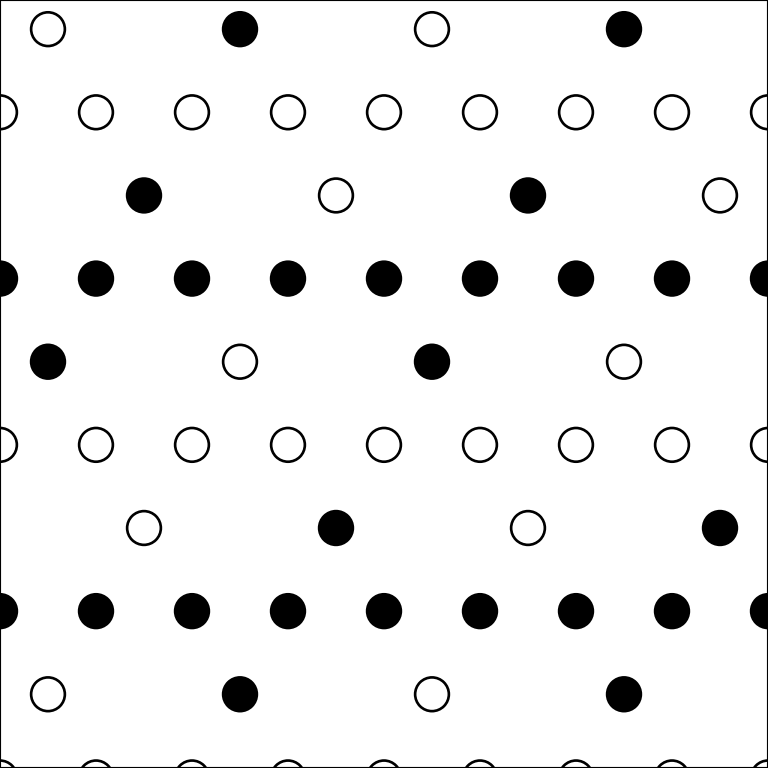

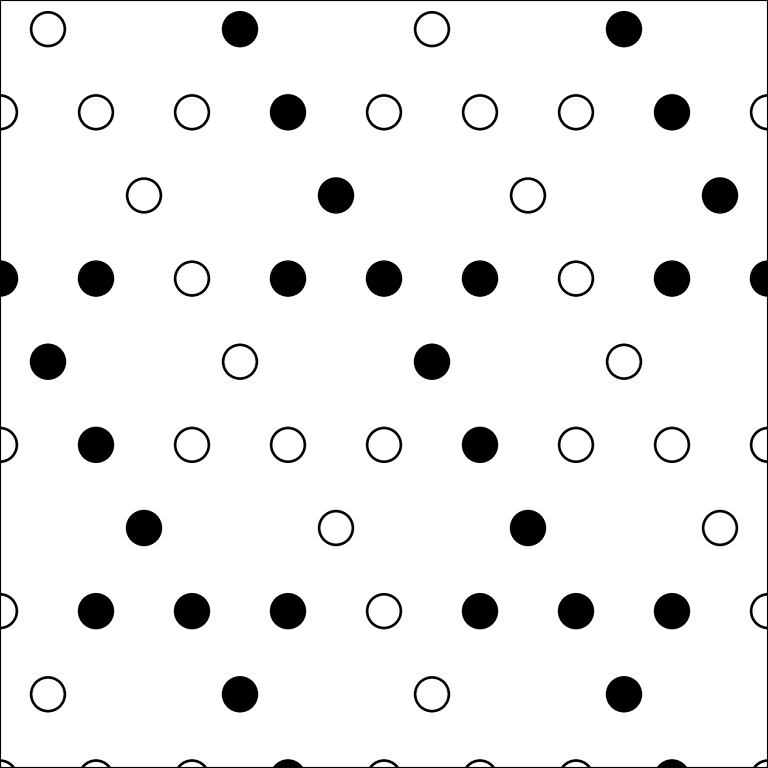

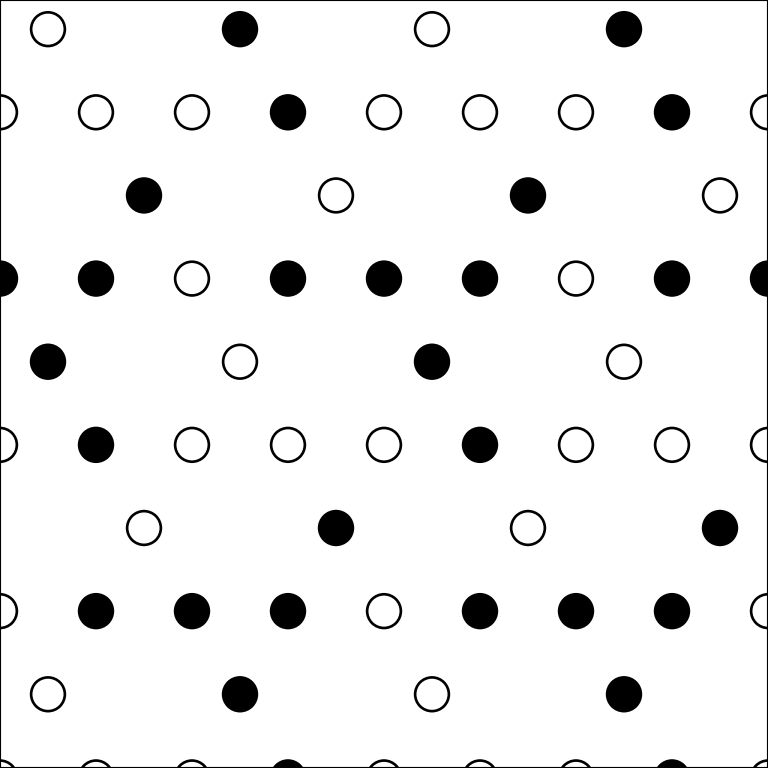

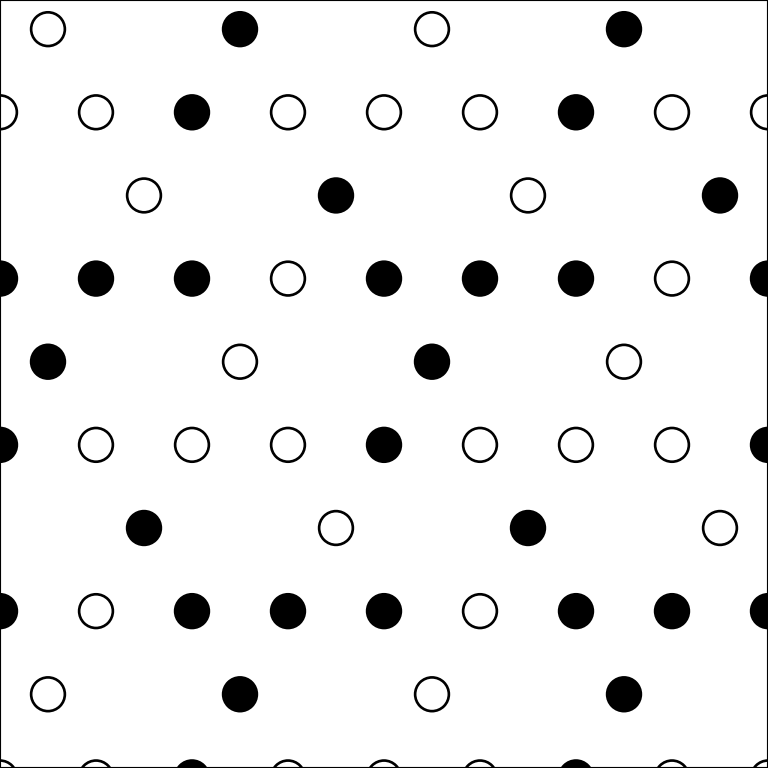

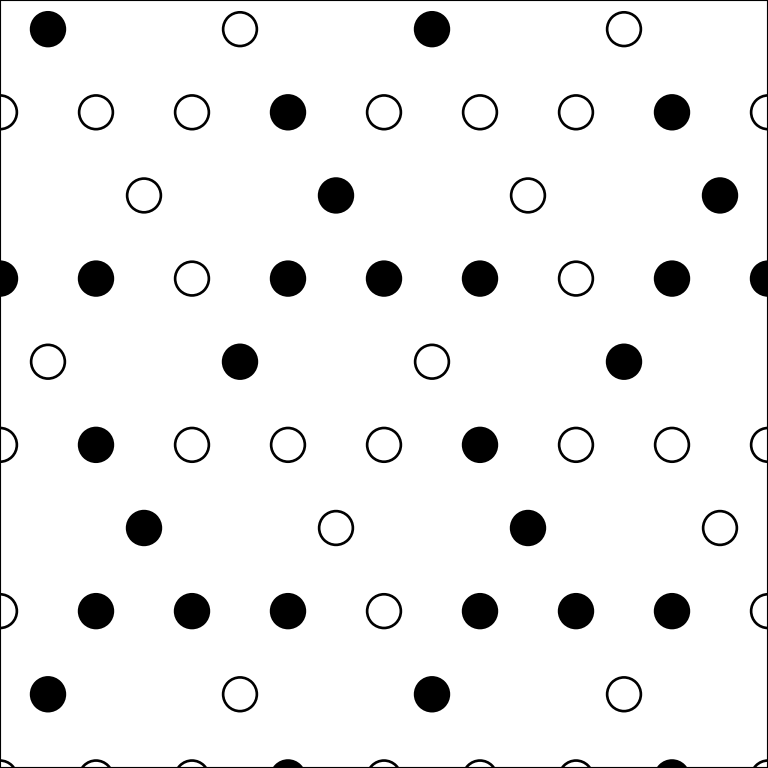

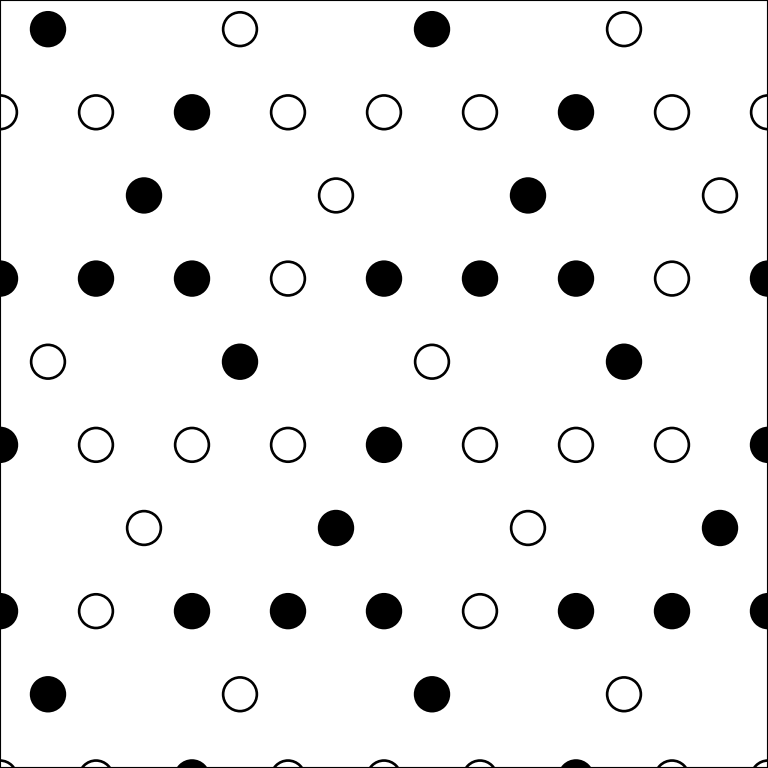

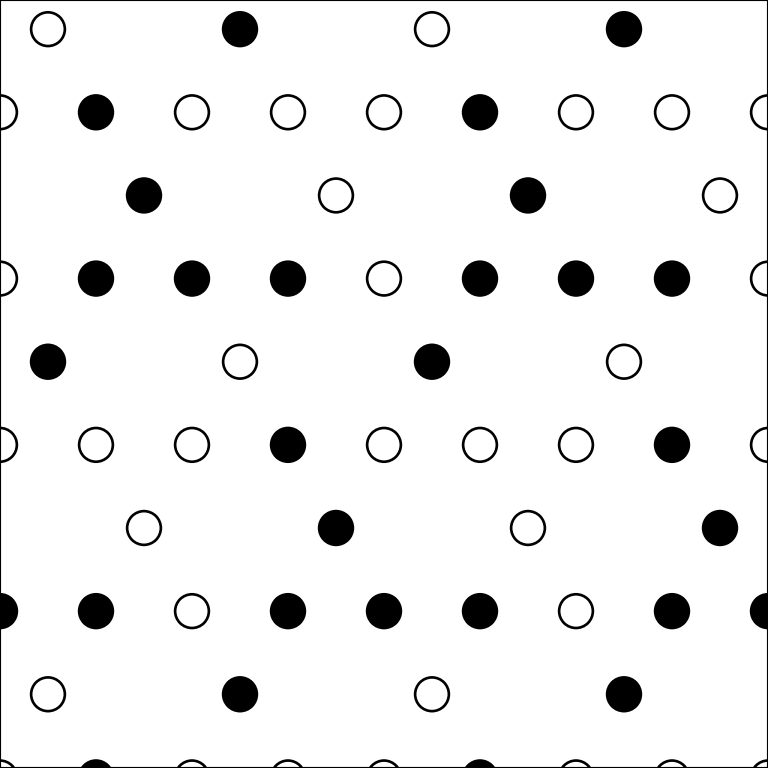



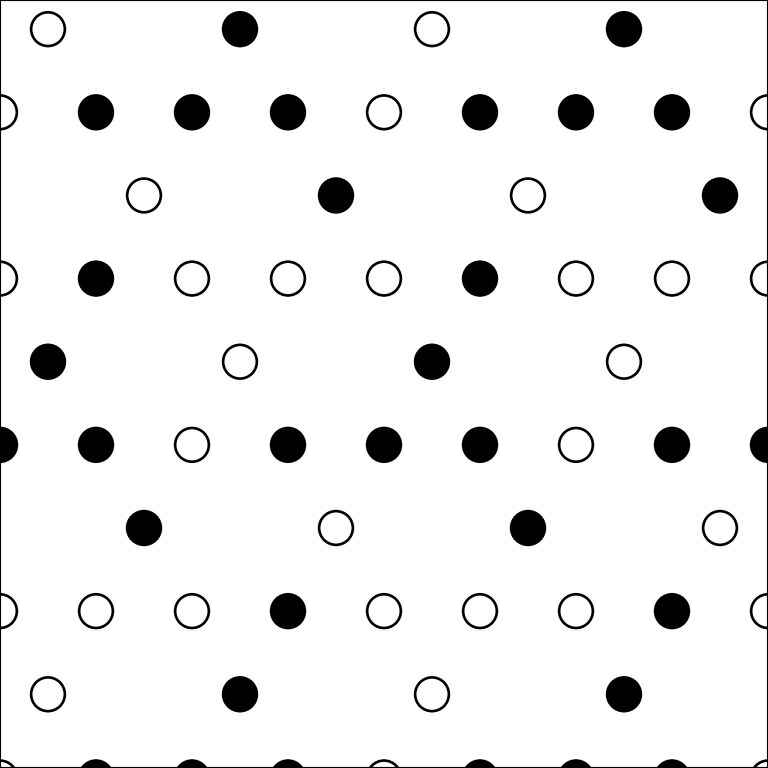

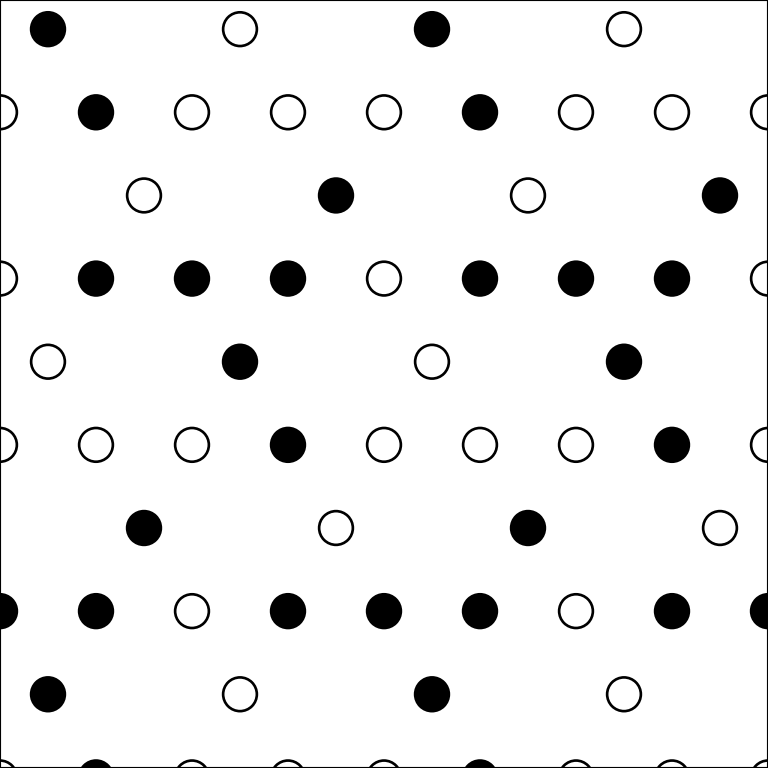

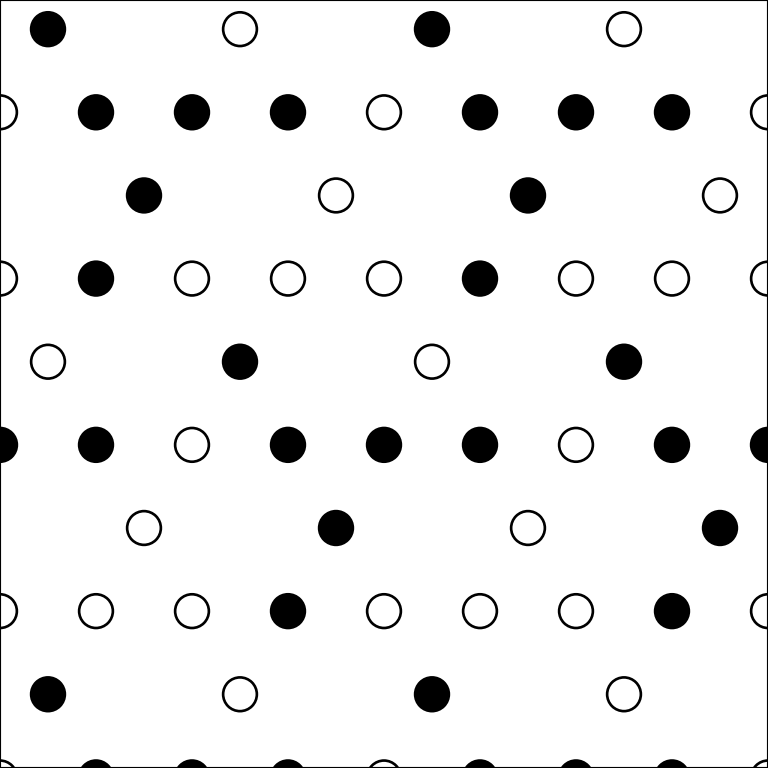

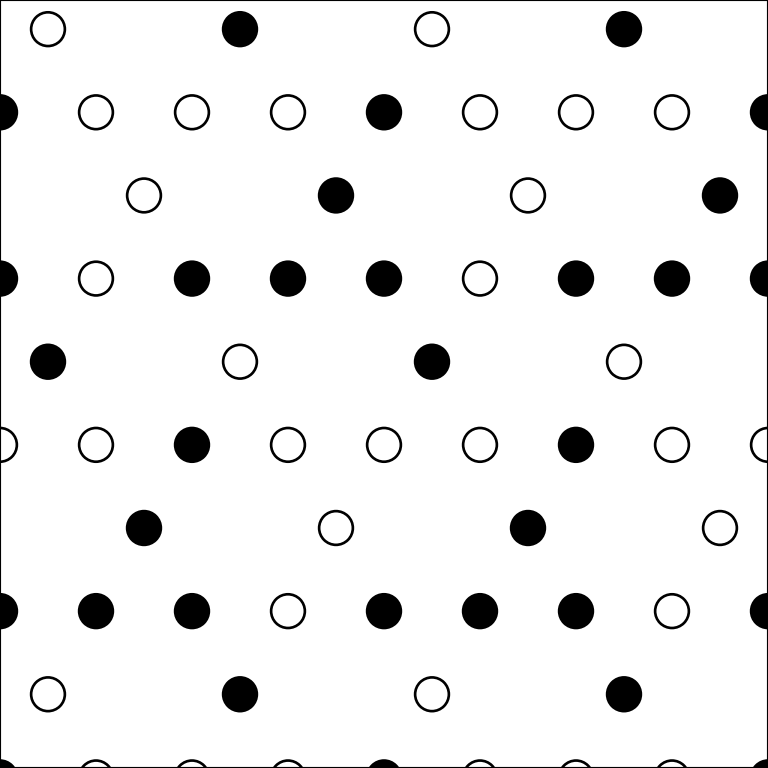

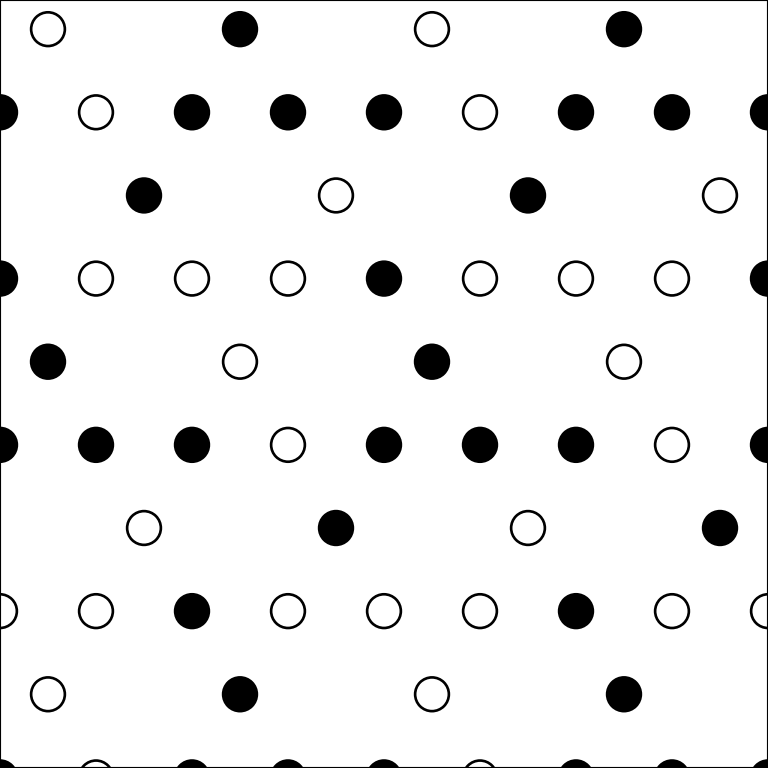

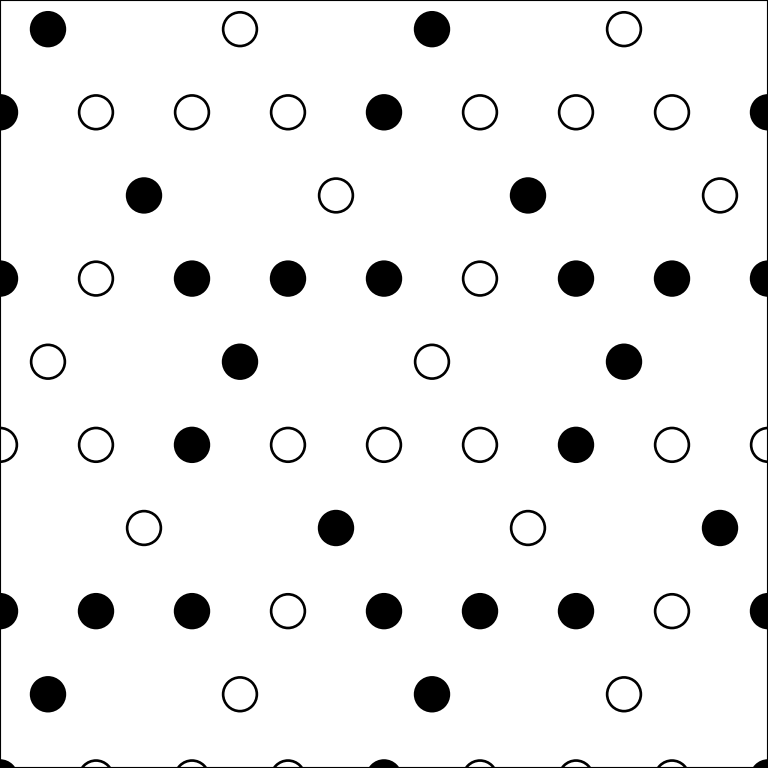

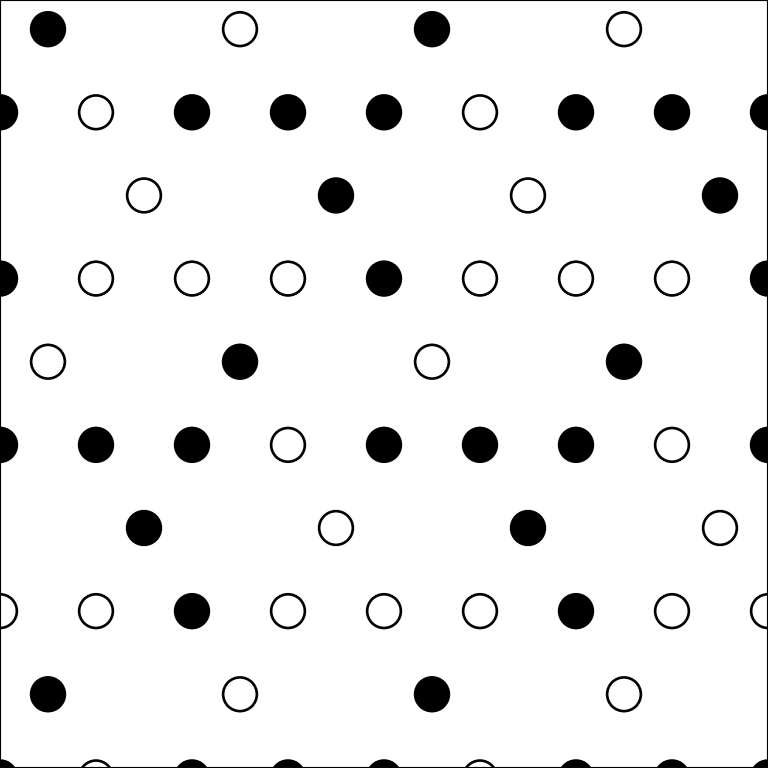

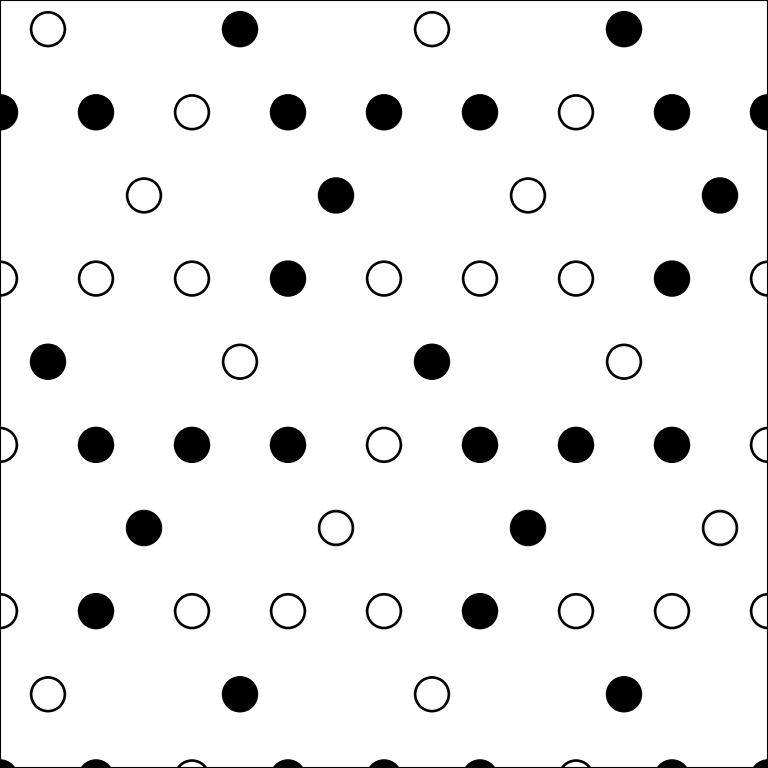



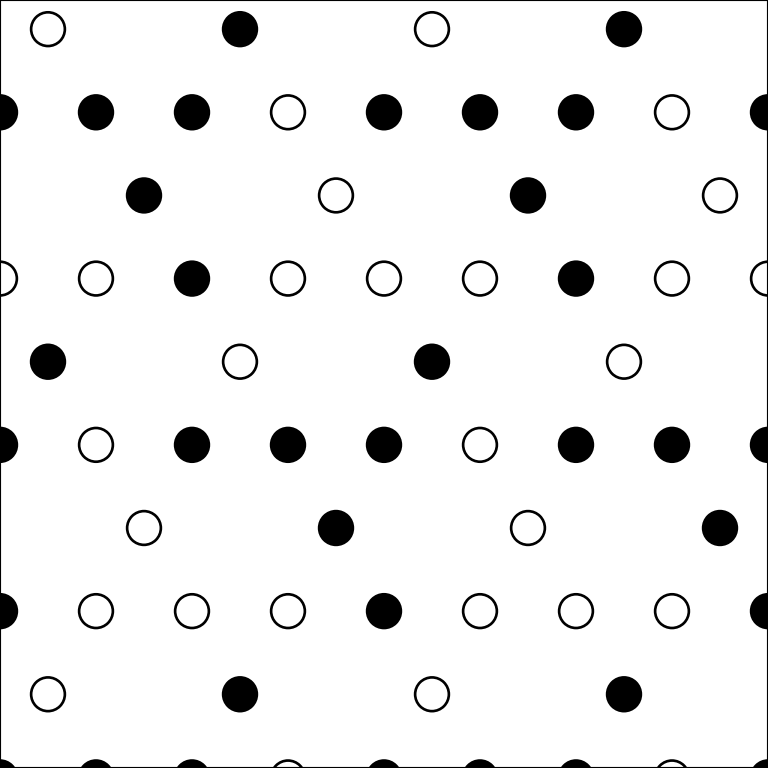

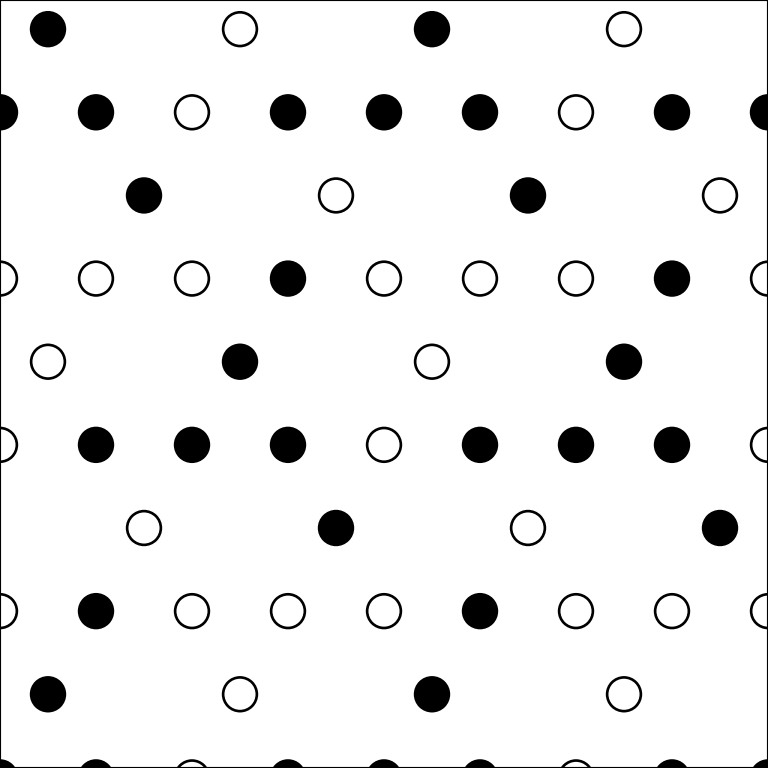

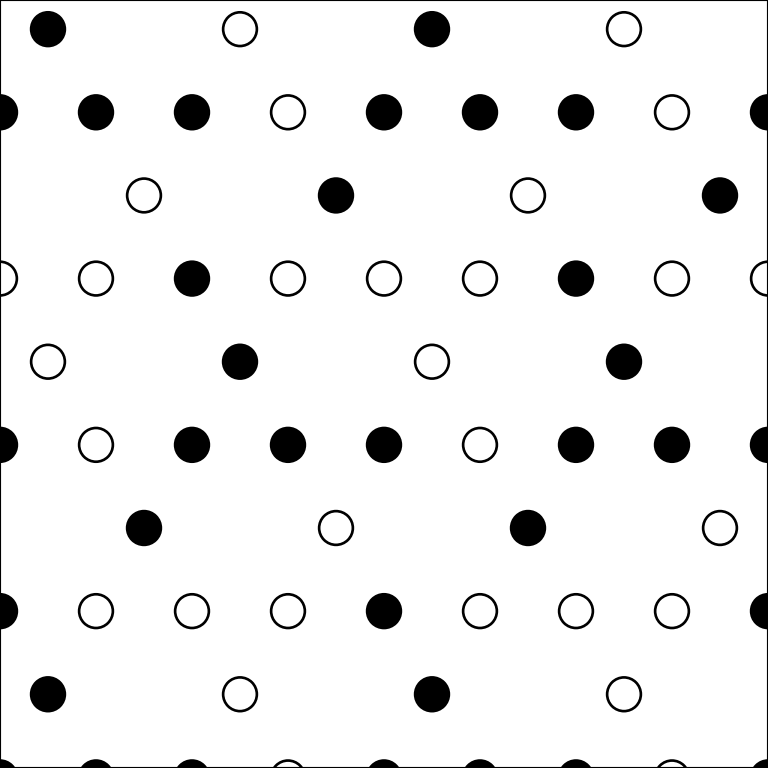

Supplement: Supplementary file 1 [file ice-configurations-12.pdf]
