# Supplementary material for: Frustration-induced emergent Hilbert space fragmentation
Source: arXiv:2011.01936 source file (2021-06-16)

component #1/20 (size: 26760). configuration #1/107176

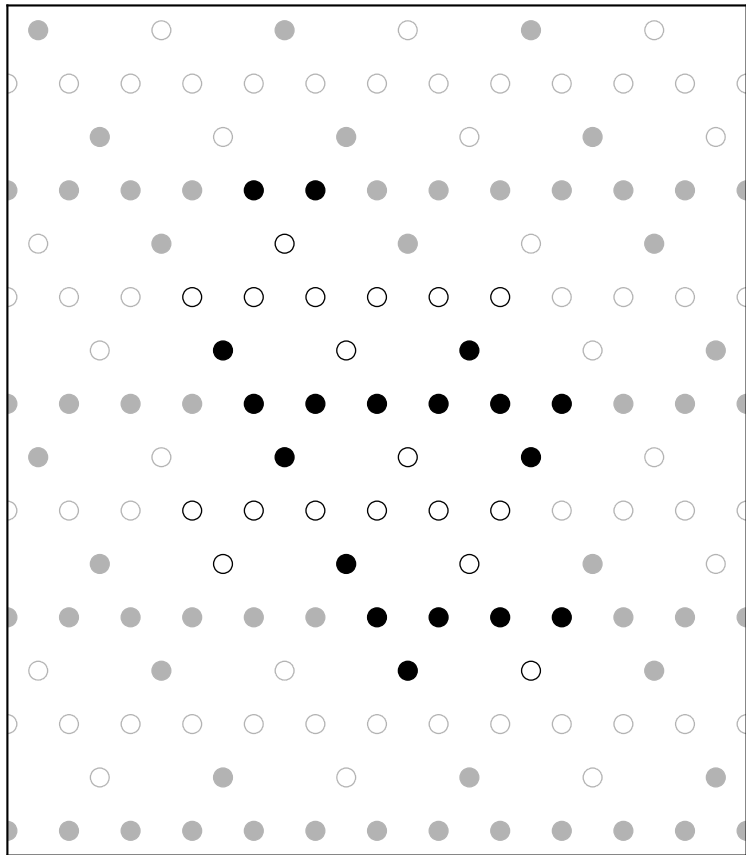

component #2/20 (size: 26760). configuration #2/107176

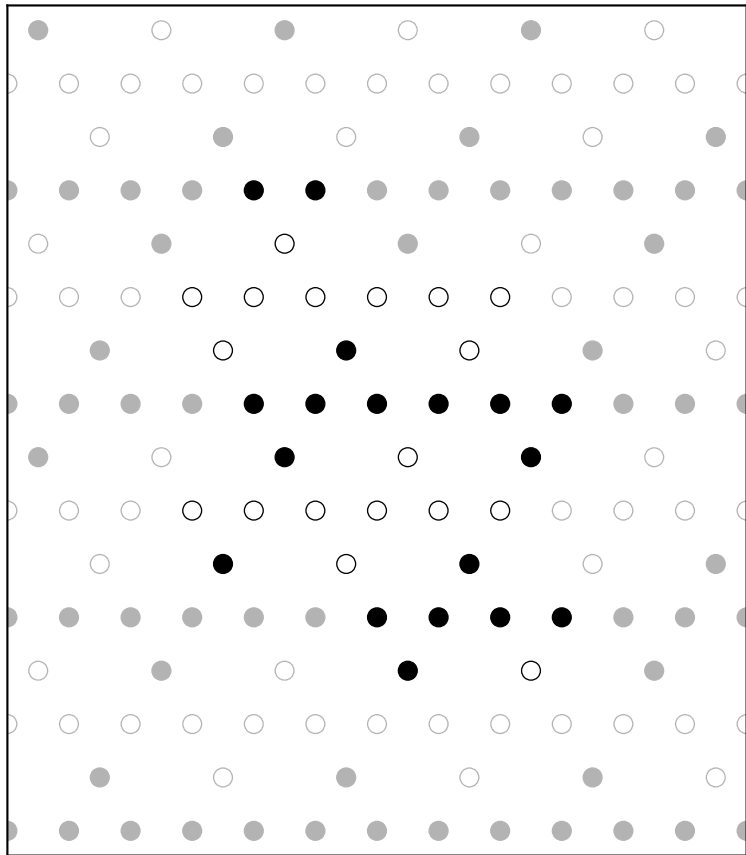

component #3/20 (size: 26760). configuration #3/107176

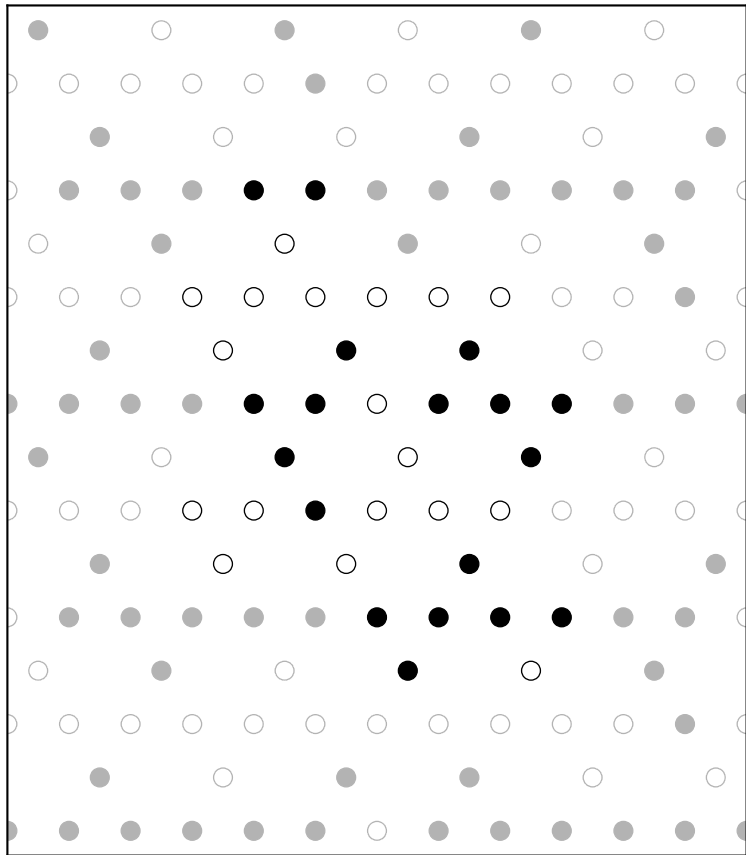

component #4/20 (size: 26880). configuration #9/107176

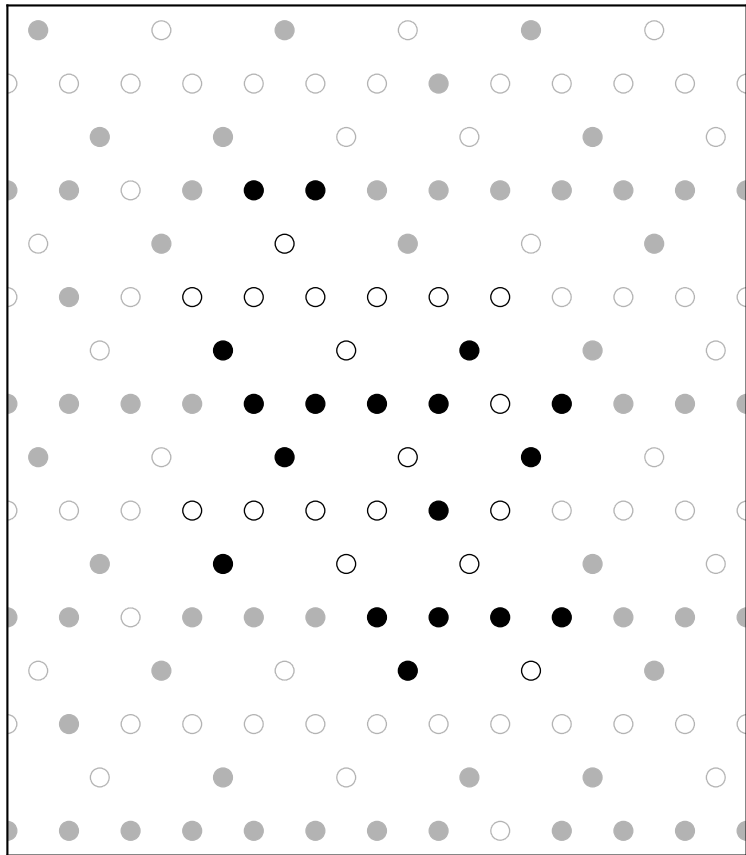

A 10x10 grid of circles, representing a 2D lattice. The circles are colored white, gray, or black. The distribution is as follows:

| Row \ Column | 1     | 2     | 3     | 4     | 5     | 6     | 7     | 8     | 9     | 10    |
|--------------|-------|-------|-------|-------|-------|-------|-------|-------|-------|-------|
| 1            | Gray  | White | Gray  | White | White | White | Gray  | White | White | Gray  |
| 2            | Gray  | White | White | White | Gray  | White | White | White | Gray  | White |
| 3            | White | Gray  | Gray  | Gray  | White | Black | Gray  | Gray  | White | Gray  |
| 4            | White | Gray  | White | White | White | White | Gray  | White | White | Gray  |
| 5            | Gray  | White | Black | White | White | White | Black | White | White | Gray  |
| 6            | Gray  | Gray  | White | Gray  | Black | Black | White | Black | Black | Black |
| 7            | Gray  | White | White | Black | Black | White | Black | Black | Black | White |
| 8            | Gray  | White | White | White | Black | White | White | White | Gray  | White |
| 9            | White | Gray  | Gray  | Gray  | White | Gray  | Black | Black | White | Black |
| 10           | Gray  | White | Gray  | Gray  | Gray  | White | Gray  | Gray  | White | Gray  |

component #6/20 (size: 1). configuration #2868/107176

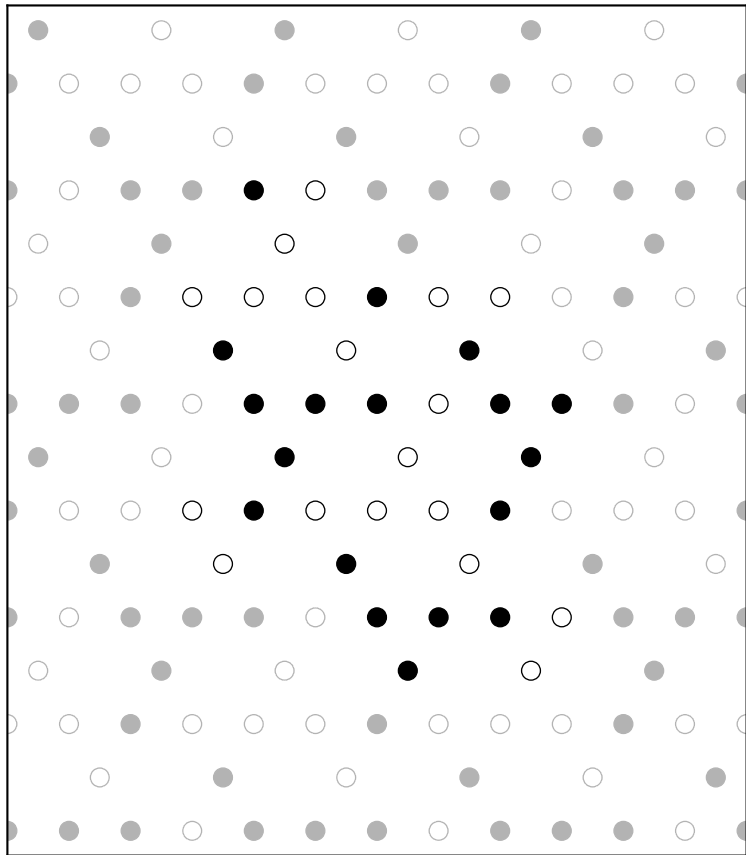

component #7/20 (size: 1). configuration #11250/107176

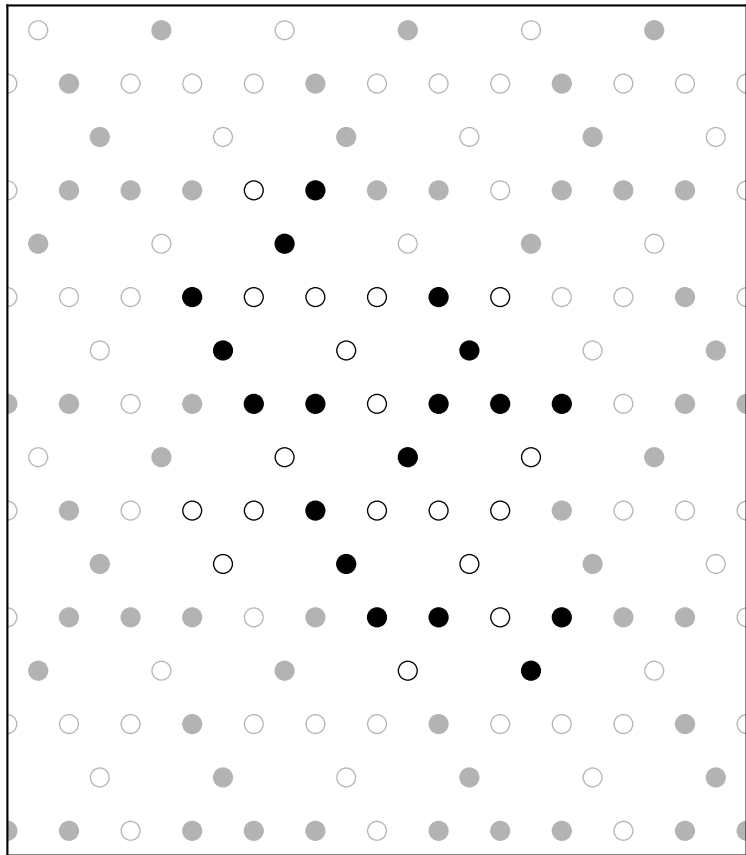

component #8/20 (size: 1). configuration #15805/107176

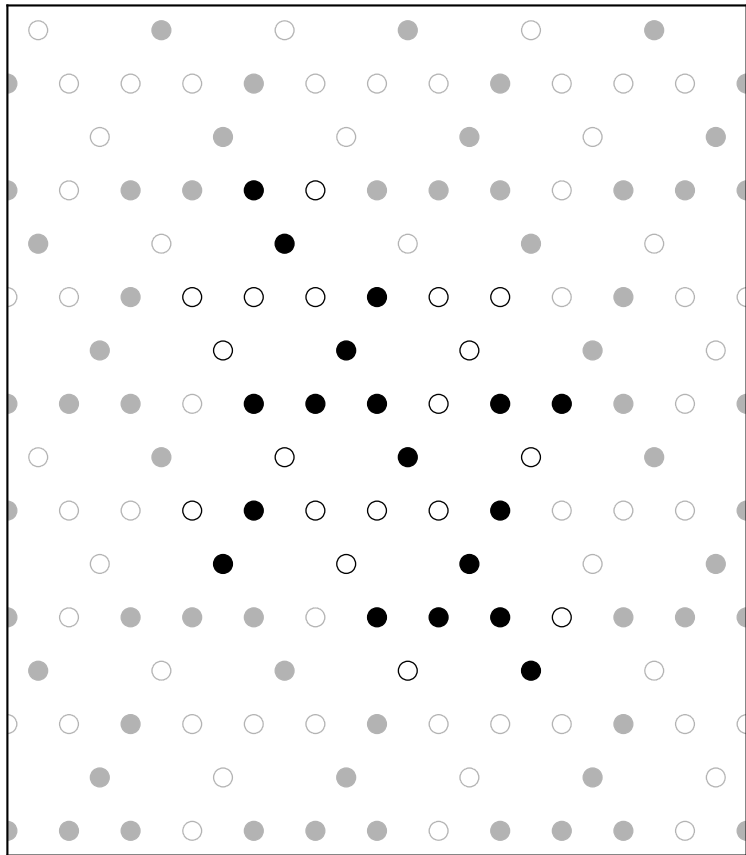



component #9/20 (size: 1). configuration #24065/107176

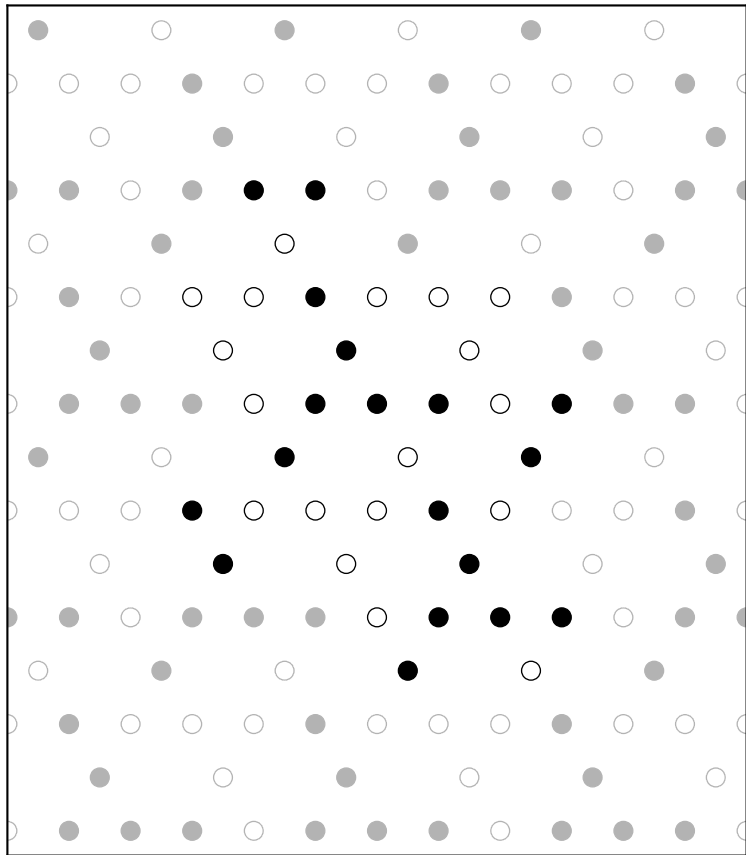

component #10/20 (size: 1). configuration #37711/107176

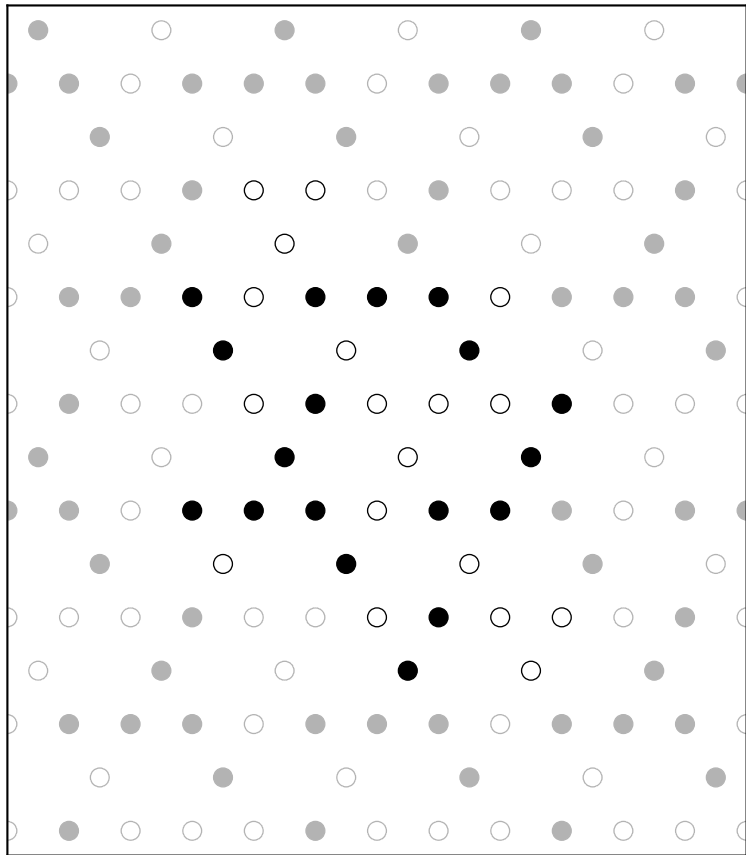

component #11/20 (size: 1). configuration #38476/107176

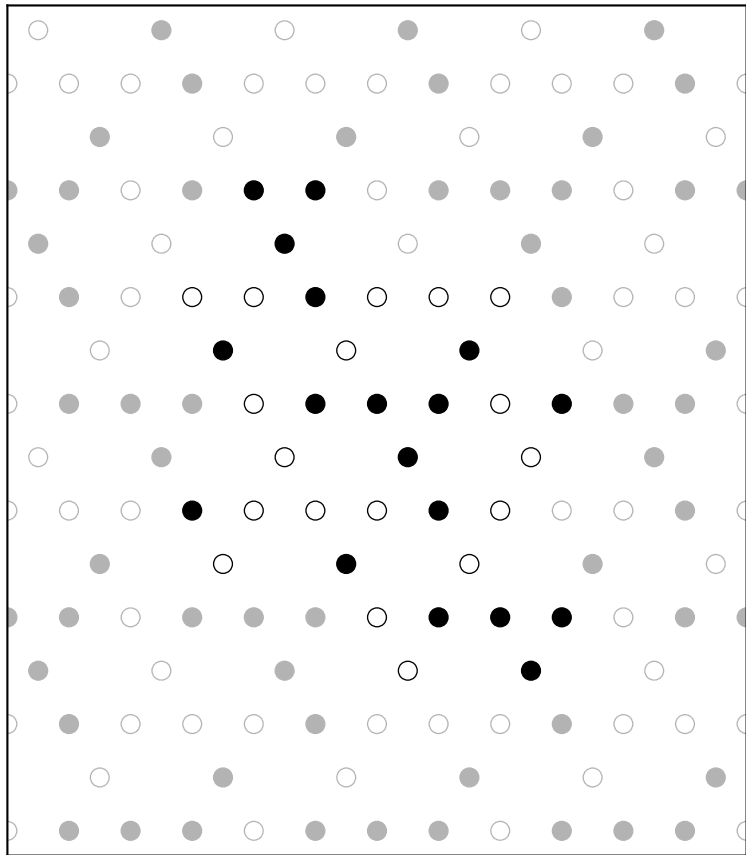



component #13/20 (size: 1). configuration #54664/107176

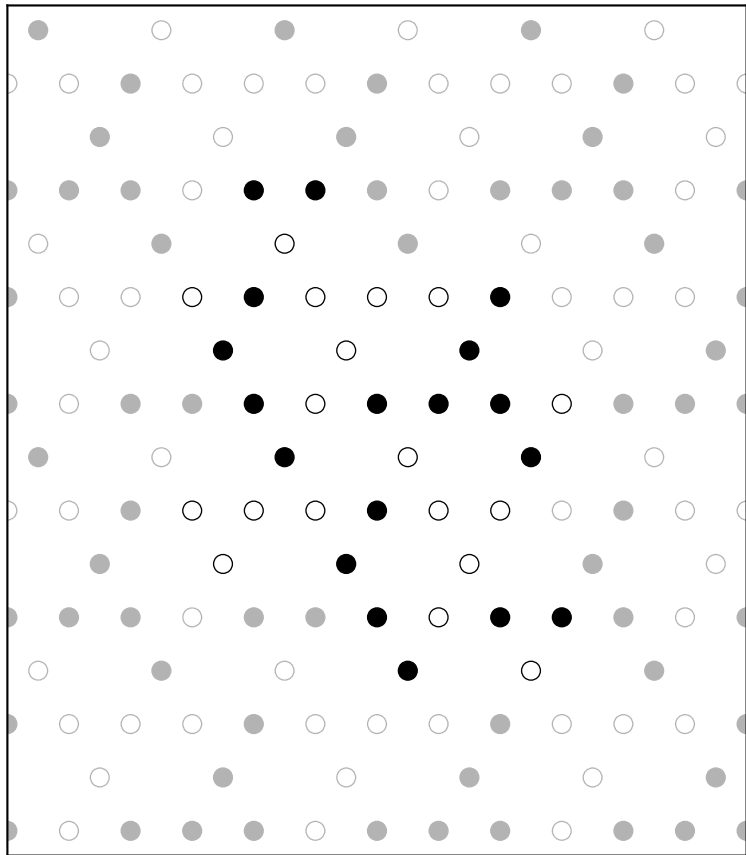

component #14/20 (size: 1). configuration #68701/107176

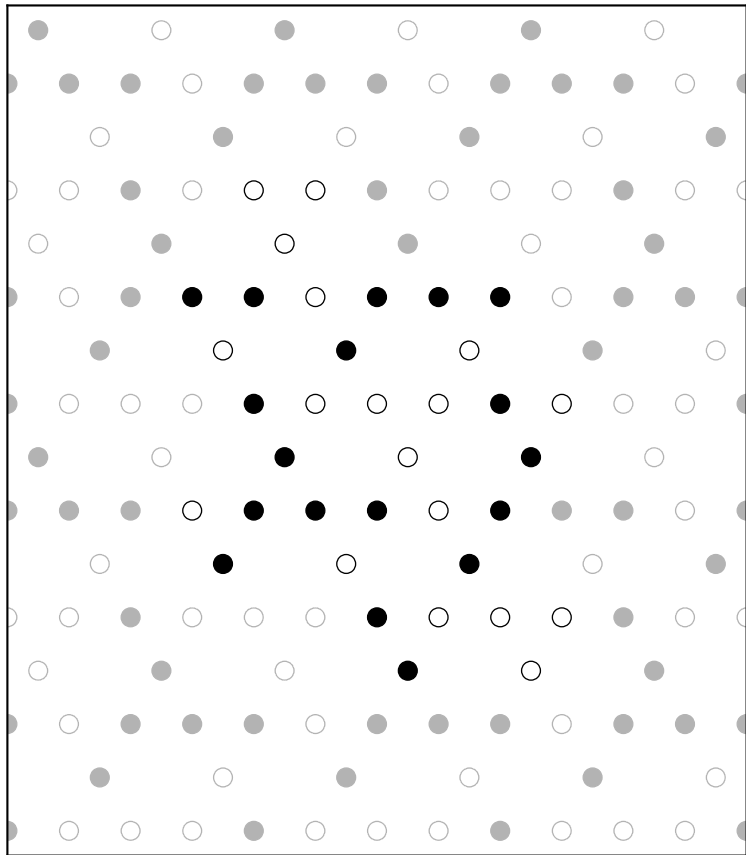

A 10x10 grid of circles, each either white, gray, or black. The grid is enclosed by a thick black border on the left and bottom edges. The distribution of colors is as follows:  
Row 1: White, Gray, White, Gray, White, Gray, White, Gray, White, Gray.  
Row 2: White, White, Gray, White, White, White, Gray, White, White, White.  
Row 3: White, Gray, Gray, White, Black, Black, Gray, White, Gray, Gray.  
Row 4: Gray, White, White, Black, White, White, White, Gray, White, White.  
Row 5: White, White, White, Black, White, Black, White, Gray, White, White.  
Row 6: Gray, White, Gray, Gray, Black, White, Black, Black, Black, White.  
Row 7: White, White, Gray, White, White, White, Black, White, White, Gray.  
Row 8: White, Gray, Gray, White, Gray, Gray, Black, White, Black, Black.  
Row 9: Gray, White, White, White, Gray, White, White, Gray, White, White.  
Row 10: White, Gray, Gray, Gray, White, Gray, Gray, Gray, White, Gray.

component #16/20 (size: 1). configuration #83112/107176

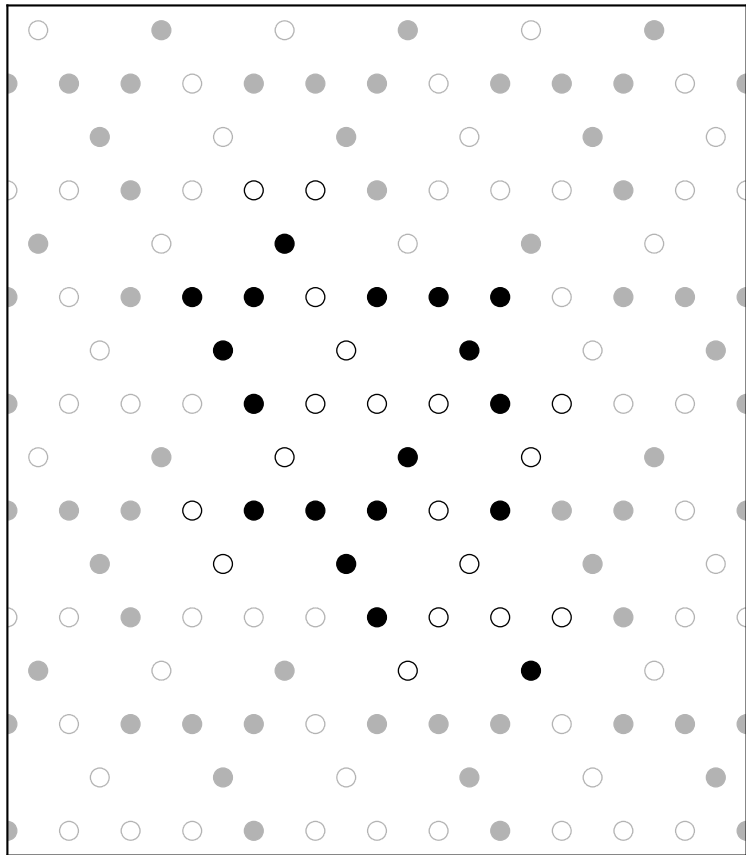



component #17/20 (size: 1). configuration #91372/107176

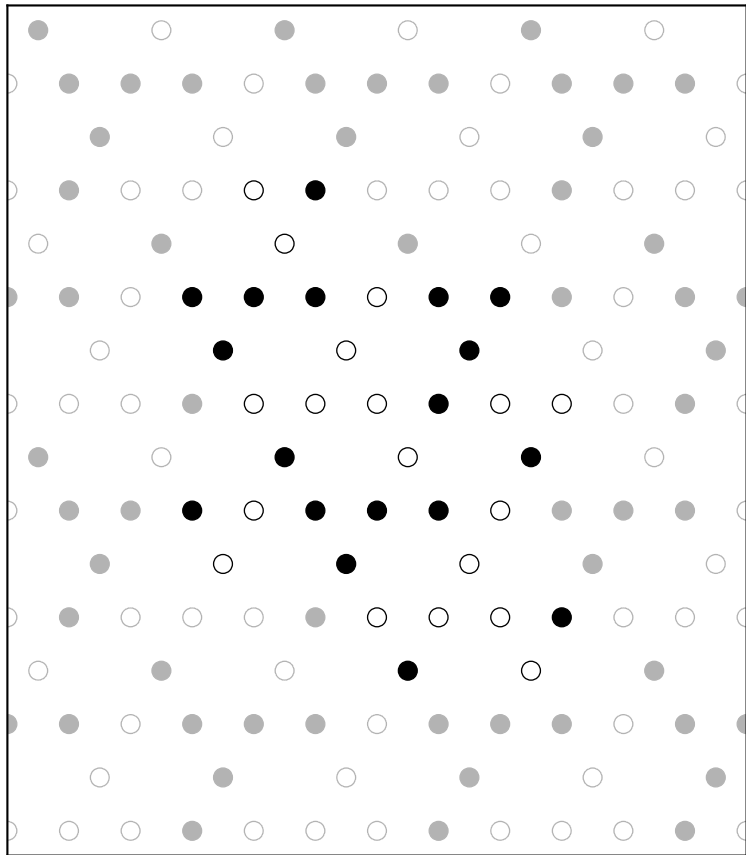

component #18/20 (size: 1). configuration #95927/107176

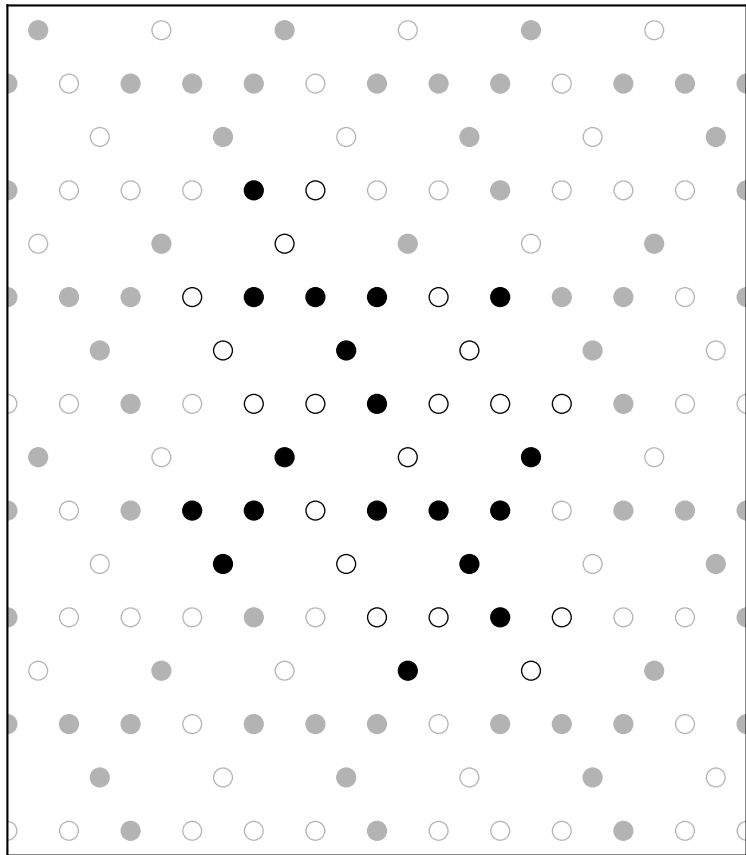

component #19/20 (size: 1). configuration #104309/107176

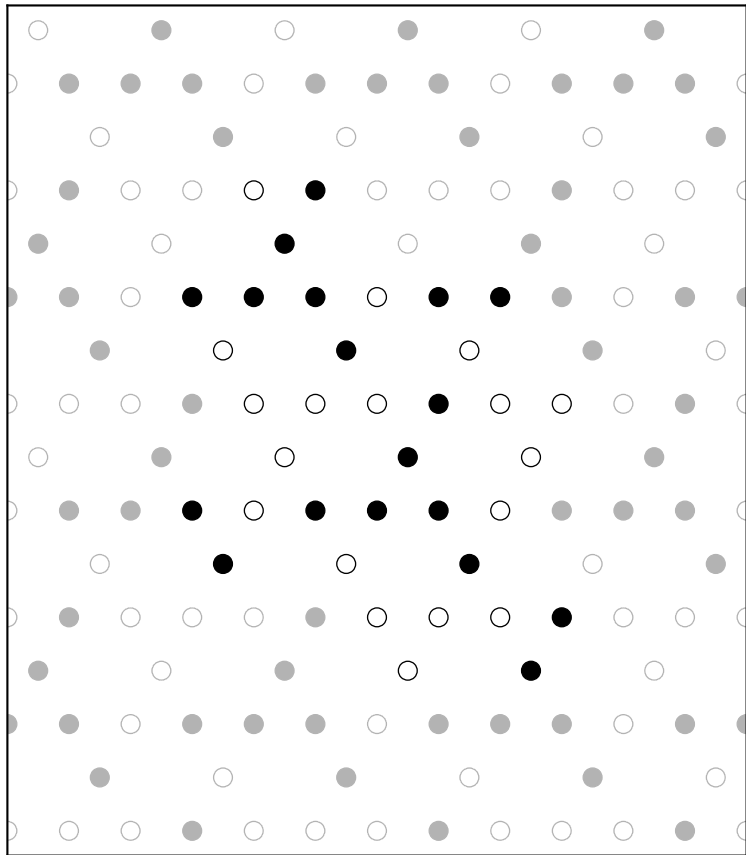

component #20/20 (size: 1). configuration #106099/107176

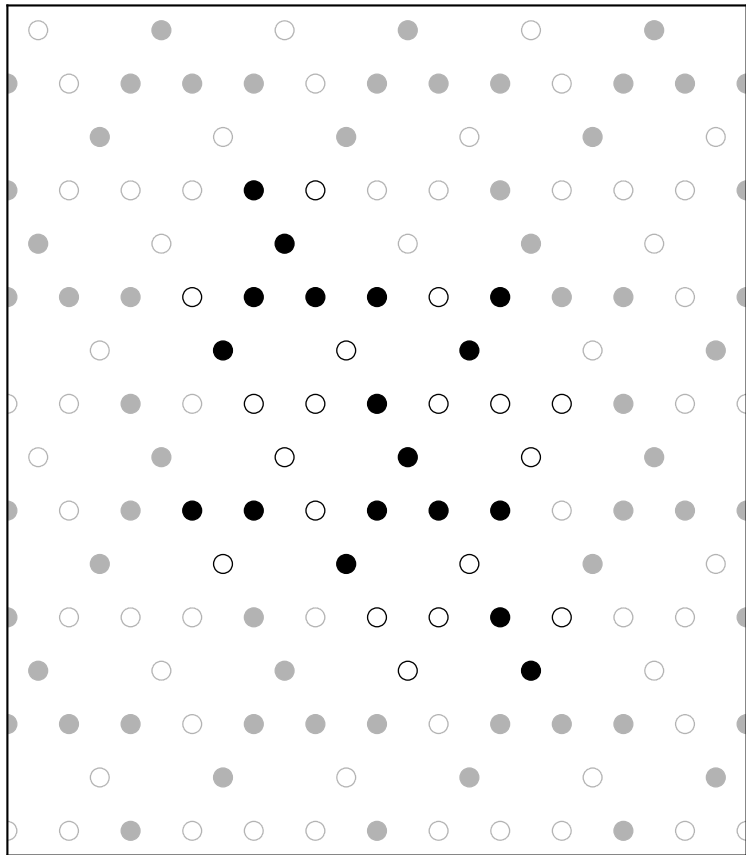

Supplement: Supplementary file 2 [file ice-configurations-36.pdf]
